# Supplementary material for: Comprehensive Structure Exploration and Thermodynamics of Graphitic Heteroatom Doped Graphene Superstructures
Source: arXiv:2509.08352 ancillary file (2026-08-20)
Supplement: Supplementary file 1 [file ESI.pdf]

# Supporting Information: Comprehensive Structure Exploration and Thermodynamics of Heteroatom Doped Graphene Superstructures

Benedict Saunders

*Department of Chemistry, University of Warwick, Gibbet Hill Road, CV4 7AL, United Kingdom*

Lukas Hörmann\* and Reinhard J. Maurer†

*Department of Chemistry, University of Warwick, Gibbet Hill Road, CV4 7AL, United Kingdom*

*Department of Physics, University of Warwick, Gibbet Hill Road, CV4 7AL, United Kingdom and*

*Faculty of Physics, University of Vienna, Vienna A-1090, Austria*

## CONTENTS

|                                                   |    |
|---------------------------------------------------|----|
| S1. DFT Convergence Tests                         | 2  |
| S1.1. K-grid convergence                          | 2  |
| S2. Formation Energy of Defects                   | 2  |
| S2.1. Chemical Potentials                         | 2  |
| S2.2. Unit Cell Size Convergence                  | 3  |
| S2.3. Formation Energy                            | 4  |
| S3. Structure prediction with SAMPLE              | 4  |
| S3.1. Sampling the Search Space                   | 4  |
| S3.2. Symmetry Reduction                          | 4  |
| S3.3. Training Set Selection                      | 6  |
| S3.4. Hyperparameter Tuning                       | 6  |
| S3.5. Training, Validation and Model Optimisation | 7  |
| S4. Gauging the Robustness of the Model           | 10 |
| S4.1. Lack of Structural Optimisation             | 10 |
| S4.2. Non-uniform Structure Generation            | 10 |
| S5. Origin of the Peak in the Heat Capacity       | 11 |
| S6. Evaluation of Thermodynamic Properties        | 13 |
| References                                        | 15 |

---

\* lukas.hoermann@univie.ac.at

† reinhard.maurer@univie.ac.at

## S1 DFT CONVERGENCE TESTS

### S1.1 K-grid convergence

For all DFT calculations, we use Generalised Monkhorst-Pack k-grids.[1, 2] These k-grids fill the Brillouin zone with an equilateral triangular mesh of k-points. The coordinate of a k-point  $\mathbf{k}$  is given by the following equation:

$$\mathbf{k} = (b_1, b_2, b_3)(\mathbf{M}^{-1})^T(n_1, n_2, n_3)^T + \mathbf{s} \quad (1)$$

Here  $b_i$  are the reciprocal lattice vectors,  $\mathbf{M}$  is a nonsingular integer matrix, and  $n_i$  are integer numbers. The matrix  $\mathbf{M}$  is optimised so that the Brillouin zone is sampled with the smallest possible number of k-points, which are separated by less than a maximum distance of  $\Delta k_{\max}$ . We converge the maximum distance between k-points  $\Delta k_{\max}$  for a sheet of pristine graphene and a sheet of carbon-nitride. We also set  $\mathbf{s}$  to zero. We find that a k-point distance of  $\Delta k_{\max} = 0.22 \text{ \AA}^{-1}$  is sufficient to attain an accuracy of 0.5 meV per atom.

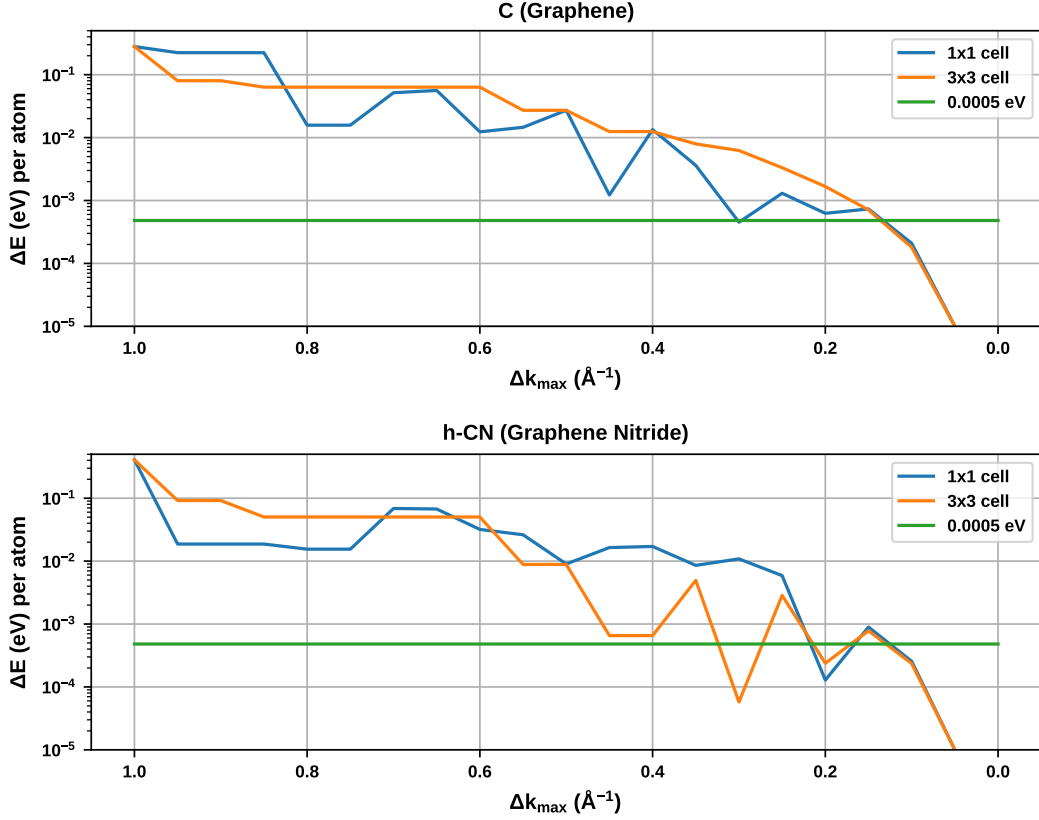

FIG. S1: Convergence of the k-grid for a 1x1 and a 3x3 unit cell of graphene.

## S2 FORMATION ENERGY OF DEFECTS

### S2.1 Chemical Potentials

Determining the formation energy of a defect requires calculating the chemical potentials of the atoms that are exchanged. In the present case, there are nitrogen and carbon. For both carbon, we use graphite as a reservoir, while for nitrogen, we use  $\text{N}_2$  molecules in the gas phase. Table S1 lists the chemical potentials that were calculated with PBE-GGA DFT.

TABLE S1: Chemical potentials for nitrogen and carbon.

| Species  | Chemical Potential (eV) | Typ of Reservoir          |
|----------|-------------------------|---------------------------|
| nitrogen | -1.491                  | $\text{N}_2$ in gas phase |
| carbon   | -1.037                  | C in bulk graphite        |

## S2.2 Unit Cell Size Convergence

To determine reliable formation energies for single defects, it must be ensured that defects do not interact with periodic images. We find that a unit cell size of (15, 15, 1), containing 450 atoms in the graphene lattice, is sufficiently large. Figures S2 and S3 show the convergence for graphitic and tri-pyridinic defects, respectively. The figures contain two curves: The line marked with dots shows formation energies if only atoms are replaced, but the lattice remains unaltered. The line marked with crosses shows the energy attained after performing a geometry optimisation, where the atoms and the unit cell were allowed to relax.

In the case of graphitic defects, we find that the geometry optimisation introduces a rigid shift of the energy. Moreover, this shift is small, not exceeding 0.04 eV. In the case of tri-pyridinic defects, we observe a much more substantial shift and a qualitative change in the shape of the convergence curve.

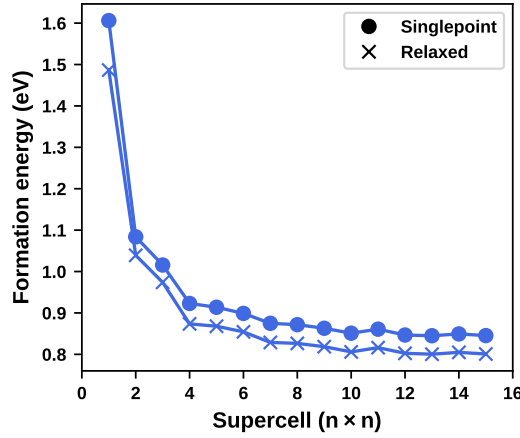

FIG. S2: Change in formation energy between the unrelaxed and relaxed lattices when introducing a graphitic defect.

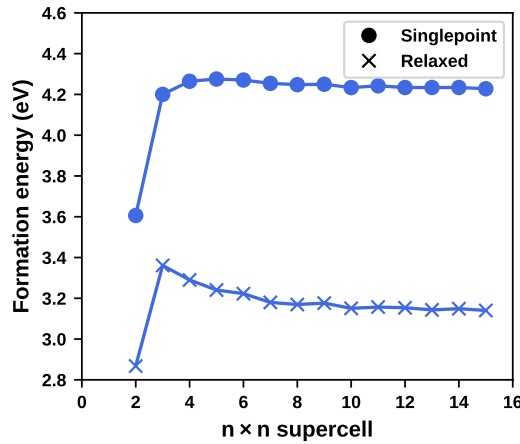

FIG. S3: Change in formation energy between the unrelaxed and relaxed lattices when introducing a tri-pyridinic defect.

### S2.3 Formation Energy

The formation energy for a graphitic and tri-pyridinic defect that we have calculated is in line with several other previous calculations from the literature, as shown in Tables S2 and S3.

TABLE S2: Literature values of the formation energies of graphitic nitrogen defects compared to the values calculated in this work. Taken from the PhD thesis[3] of Saunders with permission.

| Form. Energy (eV) | Method      | Supercell | Reference |
|-------------------|-------------|-----------|-----------|
| 0.89              | rev-vdW-DF2 | 4×4       | [4]       |
| 0.81              | PBE         |           | [5]       |
| 1.23              | PBE         | 8×8       | [6]       |
| 0.21              | PBE+D3      | 4×4       | [7]       |
| 0.86              | PBE         |           | [8]       |
| 0.87              | PBE         | 4×4       | [9]       |
| 0.96              | PBE         | 6×6       | [10]      |
| 0.80              | PBE+VdW(TS) | 12×12     | This work |

TABLE S3: Literature values of the formation energies of tri-pyridinic defects compared to the values calculated in this work.

| Form. Energy (eV) | Method      | Supercell | Reference |
|-------------------|-------------|-----------|-----------|
| 0.258             | PBE         | 4×4       | [11]      |
| 3.36              | PBE         | 4×4       | [5]       |
| 3.53              | PBE         | 4×4       | [9]       |
| 3.55              | PBE         | 8×8       | [6]       |
| 3.32              | PBE         | 6×6       | [10]      |
| 3.49              | PBE+VdW(TS) | 15×15     | This work |

## S3 STRUCTURE PREDICTION WITH SAMPLE

### S3.1 Sampling the Search Space

The configuration generation for graphitic defects is biased towards lower concentrations. Although generally such an effect does have an impact on the partition function and hence other statistical mechanics calculations, the higher concentration configurations, which correspond to larger formation energies, would only become accessible at very high temperatures. Because we are primarily interested in a temperature range from 0 K to 800 K, neglecting them is justified. The emphasis on low-concentration structures allows us to consider unit cells with a maximum of 100 atoms and to introduce up to 12 defects in more densely packed structures. An additional criterion required that any two defects be separated by at least 1.4 Å, thereby preventing defect-defect collisions. In total, this sampling scheme yields 105,614,115 configurations. Table S4 enumerates the three structure generation schemes employed to explore the graphitic configuration space from 1 to 100% nitrogen content, and for all possible supercell shapes (rectangular and skewed). For the tri-pyridinic system, a single structure generation scheme was employed, allowing the introduction of up to six defects within substrates containing up to 64 graphene unit cells.

TABLE S4: The three sampling schemes used to generate the configurations of graphitic nitrogen defects. The maximum number of defects is *not* the maximum  $\theta$  but rather is the maximum number of defects present in any generated supercell for that particular scheme.

| Scheme | Max. size of supercell (atoms) | Max. number of defects |
|--------|--------------------------------|------------------------|
| 1      | 50 (100)                       | 5                      |
| 2      | 25 (50)                        | 7                      |
| 3      | 12 (24)                        | 12                     |

### S3.2 Symmetry Reduction

The partition function of an ensemble is sensitive to duplicate structures in the dataset used to construct it. Duplicates can lead to erroneous results. Simply filtering out configurations with identical predicted formation

energies is inadequate, as it ignores genuinely distinct isoenergetic configurations. A geometry-based approach is therefore required. Figure S4 shows an example of duplicate configurations in the dataset, all predicted to be isoenergetic by SAMPLE.

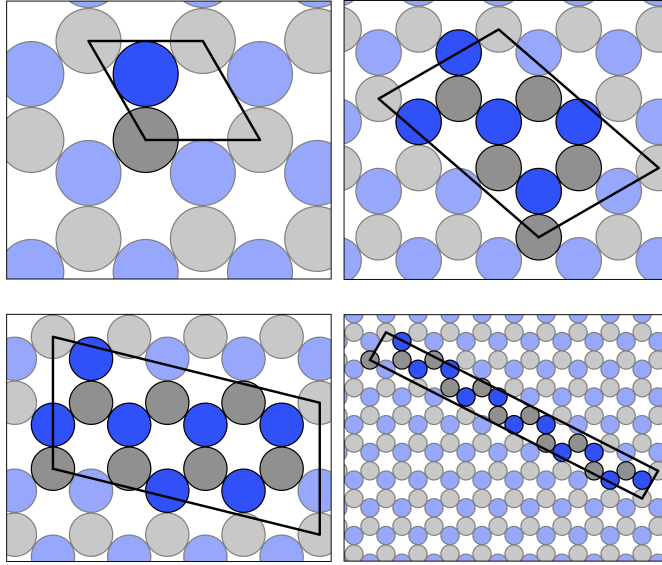

FIG. S4: Four of the nine duplicate structures found on the hull at 50% N content in the graphitic dataset. Taken from the PhD thesis[3] of Saunders with permission.

The sheer volume of data poses a substantial challenge for identifying symmetrically identical structures. However, the similarity of configurations itself is not of primary interest in this study, and therefore, similarity kernels were not employed. Even with 32-bit floating point arrays, such an approach would require more than 50 PB of memory, assuming only the upper triangular matrix is constructed. This is, of course, entirely unfeasible. Therefore, we use a two-stage symmetry reduction based on SOAP descriptors[12] and SHA-256 hashes.

Numerical noise observed between SOAP vectors of identical systems arises from the DFT geometry optimisation pre-treatment of the graphene unit cell before use in the SAMPLE models. Experimentally, perfect graphene has a unit cell with a lattice parameter of 2.464 Å and angles of 120° and 60°. However, the resulting lattice vectors do not translate into exact decimal representations and can cause slight symmetry breaking. This is not an issue when SAMPLE constructs hash representations of configurations, as a symmetry tolerance can be applied, but it becomes problematic when determining real-space distances between defects in supercell geometries.

TABLE S5: Parameters used in the construction of the SOAP vectors.

| Hyperparameter   | Value  |
|------------------|--------|
| $n_{\max}$       | 4.0    |
| $l_{\max}$       | 4.0    |
| $r_{\text{cut}}$ | 10.0 Å |
| Species          | C, N   |
| $\sigma$         | 0.15   |

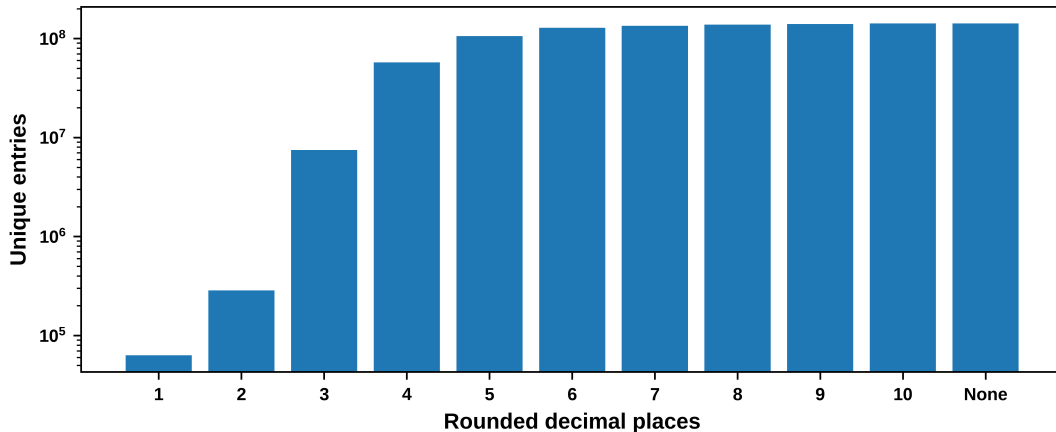

FIG. S5: The effect of rounding the SOAP vectors on the number of unique SHA-256 hashes generated from the dataset. Note that the  $y$  axis is logarithmic. Taken from the PhD thesis[3] of Saunders with permission.

Since similarity was not the focus, the SOAP vectors were constructed using the parameters in Table S5. The chosen  $n_{\max}$  and  $l_{\max}$  values are lower than typically recommended,[13] as higher values, while providing a more detailed description of local environments, greatly increase the dimensionality of the SOAP vector. This was impractical given the memory overhead of processing 162M structures. The cutoff radius  $r_{\text{cut}}$  was selected as a compromise between computational cost and accuracy of the average atomic environment, and the Gaussian smearing width was increased to 0.15 to reduce numerical noise from imperfect supercell construction. Reducing the number of basis functions or spherical harmonics alone was insufficient. Despite the high similarity between vectors, they are not exactly identical and still produce different SOAP hashes.

Rounding the terms in SOAP vectors is a simple yet effective way to reduce numerical noise and set a minimum threshold in a dataset. As shown in Figure S5, excessive rounding can lead to data loss. Using known duplicates, the SOAP vector threshold was set to  $1 \times 10^{-5}$  and validated with similar but non-identical configurations. SHA-256 hashes were then generated from the rounded SOAP vectors. Both the vectors and their hashes were stored in an HDF5 file, which provided fast access and was crucial for determining the optimal rounding threshold. The SOAP-hashing method addresses the limitation of the SAMPLE hash, which fails to identify symmetrically equivalent supercells—examples of which are shown in Figure S4, all sharing identical SOAP hashes at the  $1 \times 10^{-5}$  threshold.

A significant advantage of this approach is that it does not require explicit computation of symmetry operations and offers a much faster solution. The comparison of every symmetry operation with every other within a dataset as large as the graphitic configurations would be prohibitive. However, this method is not without its drawbacks, remaining sensitive to the selection of SOAP hyperparameters and the rounding threshold. This is particularly prominent when it comes to the cutoff radius for each of the local environments and can result in the average SOAP vector not properly capturing interactions between constituent atoms beyond this distance. However, it has recently been shown that the SOAP definition can be adapted to better describe these long-range interactions[14].

### S3.3 Training Set Selection

As conducted in previous studies using the SAMPLE method, we generate the training set using a  $D$ -optimal approach, the premise of which is to select training data to be as diverse yet feature-rich as possible. However, to make this computationally tractable, we first randomly choose a subset of 100,000 configurations from which the training set is selected. The validation set is sampled from the remaining configurations, avoiding training-validation contamination. The configurations in the training and validation sets are then subject to single-point DFT calculations, as described above.

### S3.4 Hyperparameter Tuning

Key to training a machine-learning model is the careful selection of hyperparameters and understanding the sensitivity of the model to changes in their values. SAMPLE contains two types of hyperparameters: those for which physical values can be determined and those that are purely numeric parameters.

We will first discuss physically motivated hyperparameters. The hyperparameters  $d_{\min}$  and  $d_{\max}$  were selected based on the geometry of the defect and the maximum cell size to be considered, and it follows that  $E_{\text{form}}$  is the

DFT-calculated formation energy of the defect. The graphitic defect only occupies one site. Therefore, the SAMPLE descriptor used in this model is rather simple: a 1D vector describing the frequency of each interaction at all of the distances up to  $d_{\text{max}}$ , the specified cutoff. Despite finding the interactions to be zero at distances greater than 29.6 Å,  $d_{\text{max}}$  was set at the smaller 17.0 Å for this model. This is because  $d_{\text{max}}$  is used when constructing the geometries, and 17.0 Å is the maximum non-periodic distance between sites within the pool of 452 substrates.

For the one-body prior, we use the formation energy of an isolated defect from Table S2 to inform the mean, but the standard deviation is a hyperparameter to be optimised. Interactions can be attractive or repulsive, and for this reason, the two-body prior distribution mean is set to zero, and again, the standard deviation is to be optimised. Two more hyperparameters that we keep fixed and are not subject to optimisation are the minimum and maximum separation distances; the former is inferred directly from the geometries to avoid defect collisions, and the latter is taken from our DFT calculations.

The remaining hyperparameters to be optimised are the decay distance and power, feature vector cutoff and resolution, and the artificial noise to add to the training data. To effectively tune these hyperparameters, we employed a two-stage optimisation procedure, using the root mean squared error (RMSE) of the validation set as the function to be minimised, as it provides a clear measure of how well the model performs on unseen data. Firstly, we perform coarse, manual sweeps of values across appropriately chosen ranges. Once suitable values were identified, a Bayesian Optimisation approach was used to further optimise the hyperparameters, using much finer ranges, which also accounts for any possible multicollinear relationships within the hyperparameter space. This multivariate optimisation was conducted with the `BayesianOptimization` Python library.[15] Table S6 shows the optimised values of the hyperparameters  $d_{\text{min}}$ ,  $d_{\text{max}}$ , and the means of the one- and two-body contributions were kept fixed, informed directly from the graphene geometry and DFT calculations. We find that applying manual sweeps is sufficient, and that applying the `BayesianOptimization` method did not reduce the error.

TABLE S6: Hyperparameters used for graphitic nitrogen SAMPLE model, obtained by manual sweeping. Taken from the PhD thesis[3] of Saunders with permission.

| Hyperparameter             | Optimised Value |
|----------------------------|-----------------|
| DFT noise                  | 0.002 eV        |
| $E_{\text{form}}$ st. dev. | 0.001 eV        |
| $E_{\text{pair}}$ st. dev. | 1.310 eV        |
| Correlation length         | 9.850 Å         |
| Decay length               | 1.230 Å         |
| Decay power                | -2.000          |
| Feature threshold          | $10^{-6}$       |

### S3.5 Training, Validation and Model Optimisation

The performance of the model can be examined using a learning curve. Given the scale of the complete dataset, there are inevitably going to be configurations that are unlike anything that the model has seen in the training data. Therefore, the RMSE between the DFT data and the predicted SAMPLE energies of the validation set is used as the metric of choice to demonstrate model fitness. The training set RMSE and leave-one-out-cross-validation-RMSE (LOOCV-RMSE) still provide valuable insight into the performance of the model, too, as do their maximum errors. The results are illustrated in Figure S6. As one might expect, the highest errors for all validation set-based metrics occur for a training set with a single configuration, which then rapidly decreases upon the addition of more configurations into the training set. The significant fluctuations presented by the learning curve are expected as the model proceeds through cycles of overfitting and underfitting as new data is added.

Once the model begins to equilibrate and plateau after training on 150 structures, the RMSE of the validation data consistently remains lower than that of the training data. Additionally, the LOOCV-RMSE exhibits a gradual, albeit slight, decrease as the training set size increases. The validation set RMSE reaches a minimum of 0.0212 eV per defect at a training set size of 520 configurations. However, a marginal increase to 0.0216 eV per defect is observed at 600 configurations, which may signal the onset of overfitting. This interpretation is supported by the fact that both the training set RMSE and LOOCV-RMSE continue to decrease within the same interval of training set sizes. An overview of the final uncertainties in the model for all energy predictions of graphitic defect superstructures is provided in Table S7.

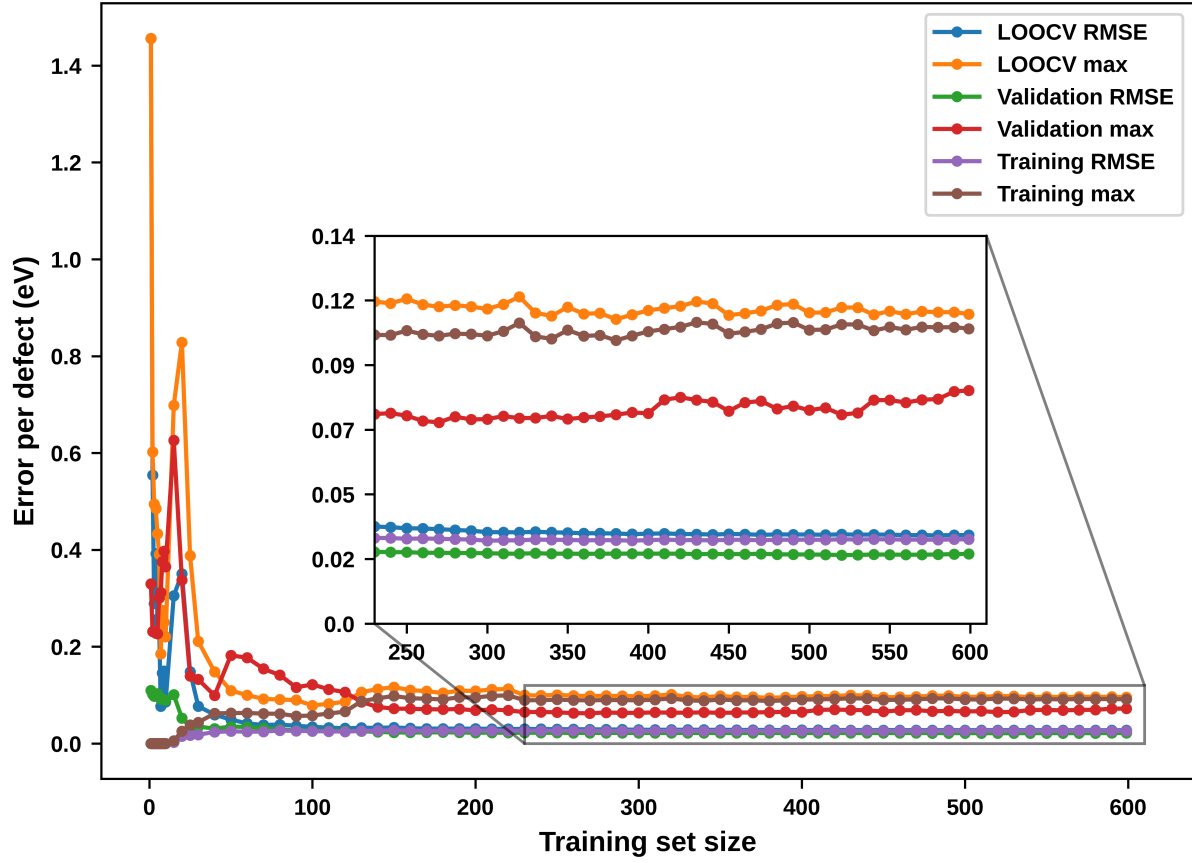

FIG. S6: The learning curve of the SAMPLE model for graphitic nitrogen defects. The configurations for each point along the  $x$  axis are  $D$ -optimally selected. Taken from the PhD thesis[3] of Saunders with permission.

TABLE S7: The errors associated with the graphitic nitrogen model. Taken from the PhD thesis[3] of Saunders with permission.

| Error                     | Quantity (eV) |
|---------------------------|---------------|
| Training RMSE             | 0.0261        |
| Training max err.         | 0.0913        |
| $R^2_{\text{Training}}$   | 0.9885        |
| Validation RMSE           | 0.0216        |
| Validation max err.       | 0.0722        |
| $R^2_{\text{Validation}}$ | 0.9888        |
| LOOCV-RMSE                | 0.0274        |
| LOOCV max err.            | 0.0958        |

The parity plot comparing the SAMPLE predictions to DFT-calculated formation energies, shown in Figure S7, demonstrates good agreement for both the training and validation datasets. All data points closely align with the ideal parity line, indicating that the model reliably reproduces the reference DFT values across the entire range of energies. No outliers are observed, suggesting that the SAMPLE approach captures the underlying physics.



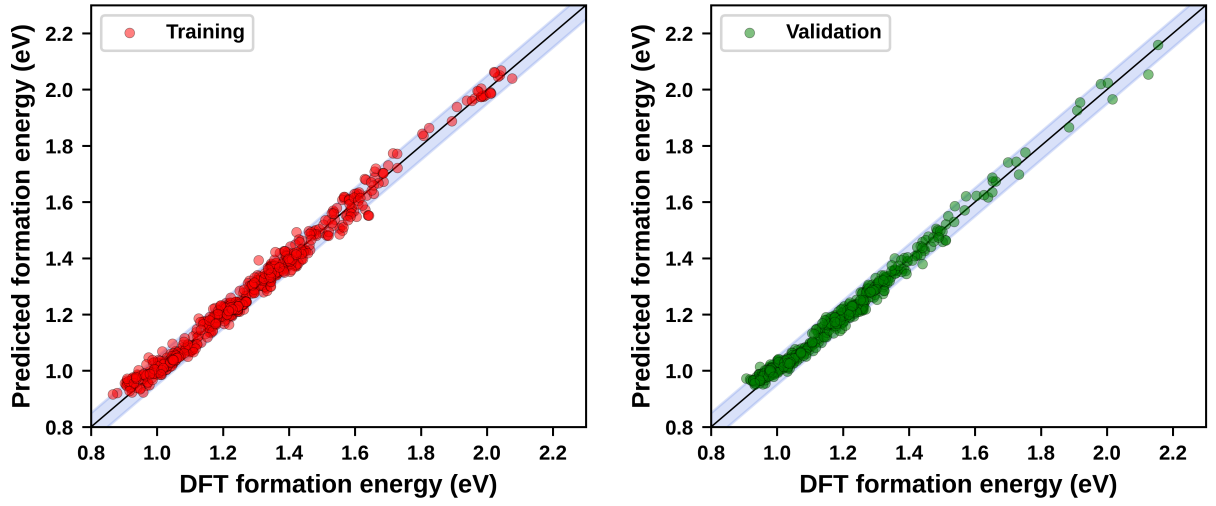

FIG. S7: Parity plots of the SAMPLE predictions for the training (a) and validation (b) sets against the DFT data for graphitic nitrogen; Left) Training set parity; Right) Validation set parity. Taken from the PhD thesis[3] of Saunders with permission.

Finally, Figure S8 shows all configurations ranked by their energy. The energy distribution shows an S-like shape, which is common for configurations generated with SAMPLE.[16–19]

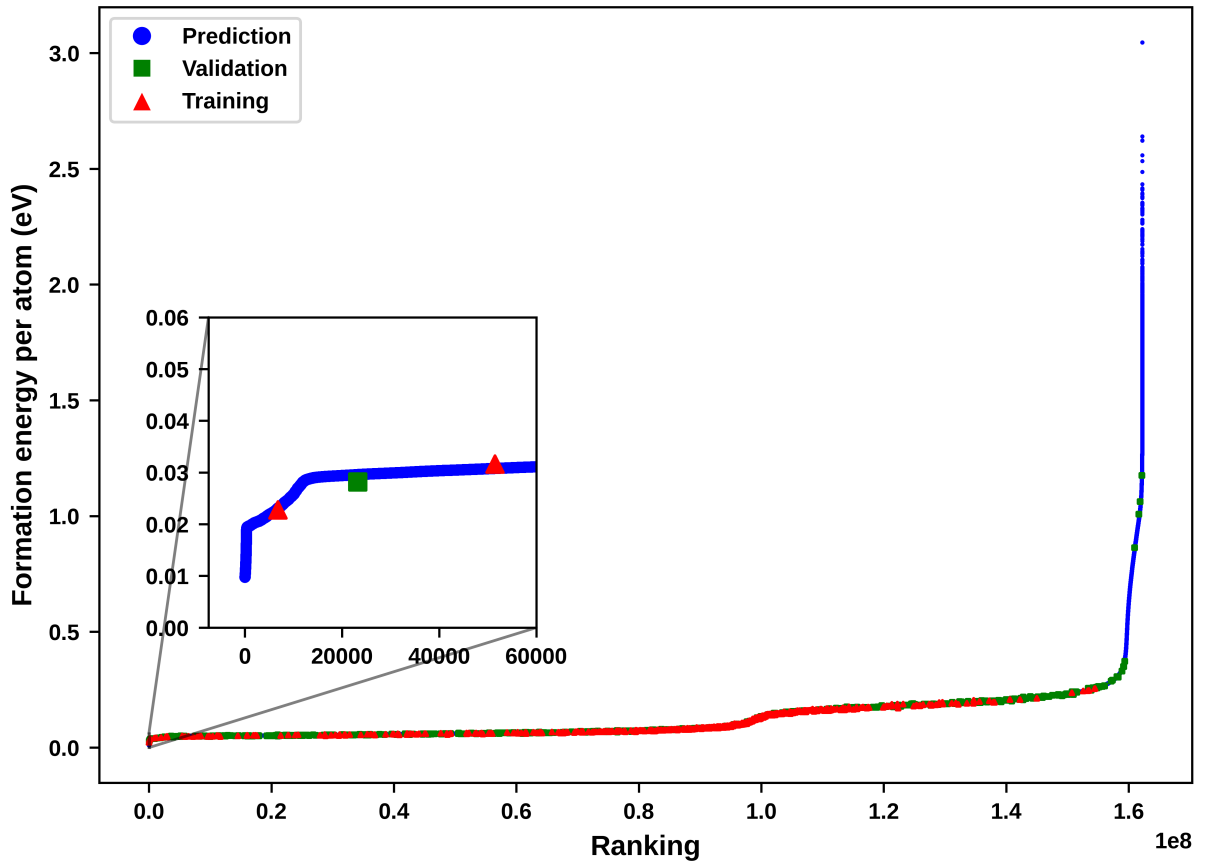

FIG. S8: Energy distribution for all 105 million structures of graphitic NDG.

## S4 GAUGING THE ROBUSTNESS OF THE MODEL

The two main approximations taken are the lack of structure optimisation and the sampling scheme. Here we will gauge the effect of these approximations on the results.

### S4.1 Lack of Structural Optimisation

A limitation of applying the SAMPLE method to substitutional defect structures is that it does not account for the relaxation of the structure when the defect is created; the spatial arrangement of lattice sites is unchanged, and the geometry remains identical to that of pristine graphene. In the case of graphitic nitrogen, we have shown using DFT calculations that there is a small, near-constant shift in energy upon relaxation (see Figure S2). The covalent radii of carbon and nitrogen are similar enough that structural optimisation does not significantly impact the geometry qualitatively, particularly for configurations with lower N content. Therefore, we expect that the lack of relaxation does not significantly affect the ranking and thermodynamics of graphitic nitrogen-defect superstructures at medium to low concentrations. However, nitrogen (hexagonal nitrogen) is a theoretical 2D allotrope of nitrogen that has been predicted to buckle, instead of lying flat like graphene.[20] Islands of nitrogen have extremely unfavourable formation energies. Therefore, uncertainties introduced in this energy are not expected to affect the results presented in this work.

This argument cannot be made for tri-pyridinic defects, for instance. As shown in Figure S3, geometry optimising these structures leads to significant energy gains and changes in relative stability of defect pair configurations, which could not be neglected when determining thermodynamic properties.

### S4.2 Non-uniform Structure Generation

Our structure generation methods are biased towards those with lower defect concentrations, as these have lower formation energies and will dominate the thermodynamics at the temperature range (0 K to 800 K) we are interested in. We have imposed an absolutely maximum of 12 nitrogen defects within any given configuration. This means, for example, that the largest configuration that can achieve a 50% defect concentration comprises of 12 graphene unit cells, i.e. 24 atoms, etc. The largest systems permitted have 100 atoms, and are responsible for the majority of the 105M configurations, as a result of the huge number of symmetrically unique ways to arrange even a small number of defects in a lattice of this size.

To gauge if this bias in the sampling affects the thermodynamics, we determine the canonical heat capacities. Hereby, each concentration becomes a separate canonical ensemble, eliminating the sampling bias. Unlike the heat capacity in the grand canonical ensemble, the heat capacity in the canonical ensemble is derived from the variance of internal energies for a fixed composition  $\theta$  at a given temperature  $T$ :

$$C_V = \left( \frac{\partial U}{\partial T} \right)_V \quad (2)$$

The canonical ensemble is evaluated using the internal energies  $U = \langle E \rangle$ . The canonical partition function is determined using the following equation:

$$Z = \sum_i e^{-\beta[\epsilon_i + \theta_i \cdot (\mu_C - \mu_N)]}, \quad (3)$$

Here  $\epsilon_i$  is the formation energy per atom predicted by SAMPLE, which already contains the chemical potentials. Therefore,  $\theta_i \cdot (\mu_C - \mu_N)$  must be added again to evaluate the canonical partition function.

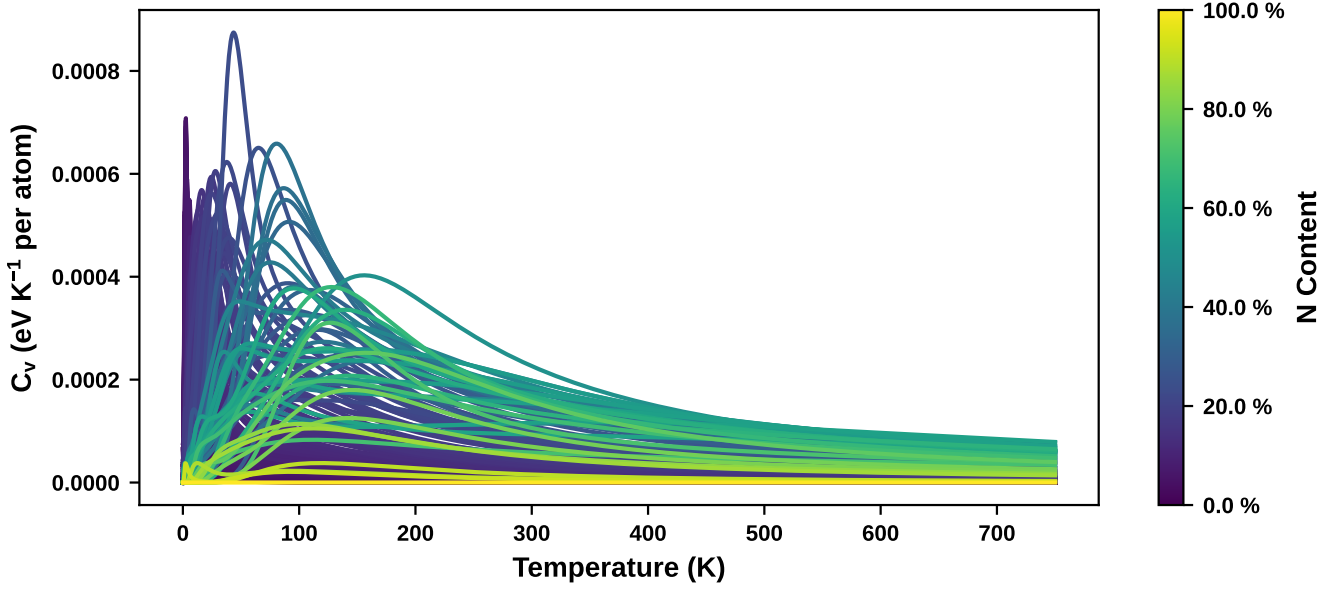

FIG. S9: Canonical heat capacities of the system energies, treating each  $N$  as its own ensemble. Taken from the PhD thesis[3] of Saunders with permission.

Peaks are also observed in the canonical heat capacities for all concentration values, as shown in Figure S9. This confirms that the peak in the grand canonical heat capacity is not an artefact of the structure generation method. No peaks are observed in the heat capacity for the system with 100% nitrogen content. In this case, the system is fully saturated with nitrogen, meaning no other configurations can exist that could be thermodynamically accessed. Additionally, several canonical heat capacities exhibit multiple maxima, particularly at low temperatures ( $T < 40$  K). Some of these double-peak heat capacities even occur in systems where the nitrogen concentration  $\theta$  exceeds 75%.

At higher concentrations, the peaks shift to higher temperatures. As the grand canonical heat capacity can be roughly approximated as a weighted accumulation of the canonical heat capacities, additional high concentration configurations can shift the peak upwards. However, thermal occupation strongly favours low concentration configurations, limiting this effect.

## S5 ORIGIN OF THE PEAK IN THE HEAT CAPACITY

Peaks in the heat capacity have been observed in multiple systems and attributed to various system properties, as we discuss in the Discussion in the main manuscript. To determine the origin of the peaks, we have constructed a toy model where we generate ensembles with arbitrary energy distributions (see Figure S8). For each of these ensembles, Figure S10 illustrates the heat capacity and the ranking plot.

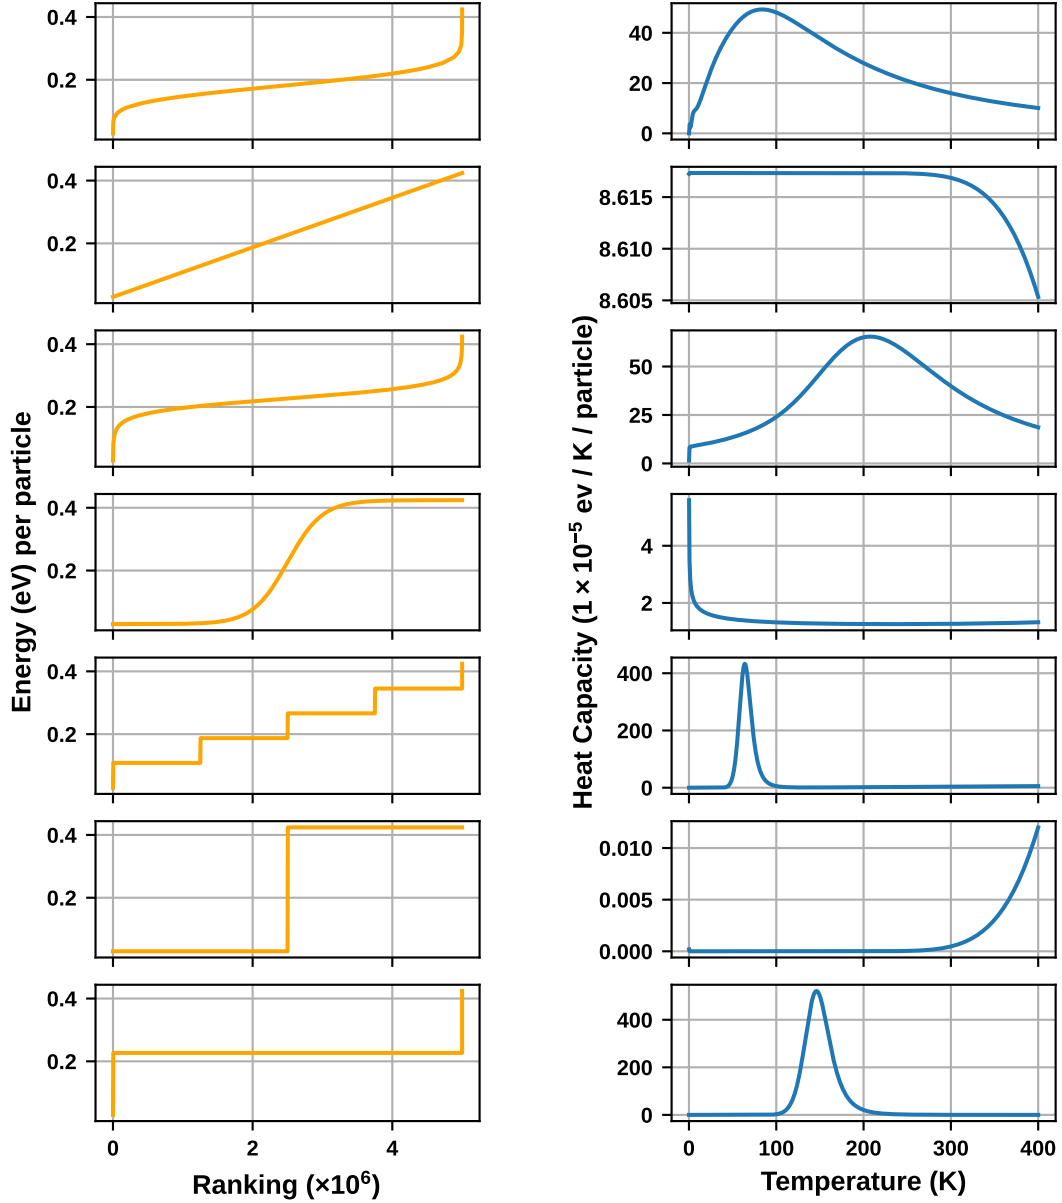

FIG. S10: The effect of various ensemble energy distributions on the specific heat capacity, assuming a canonical ensemble. From top to bottom: A charge colloid mode with randomly generated point clouds, a linear energy distribution, a logit curve, a sigmoid curve, and three different step functions.

An ensemble with a purely linear ranking plot produces a flat heat capacity without peaks. We note that the decay of the heat capacity of the linear energy distribution in Figure S10 is a finite-size effect. Introducing steps into the energy distribution gives rise to peaks in the heat capacity. The position and shape of the peaks depend delicately on the shape of the energy distribution. We note in passing that for two energy distributions, the peaks lie outside our temperature range.

The emergence of a peak in the heat capacity is governed by the shape of the energy distribution, which in turn reflects the underlying energetics of the system. One might therefore assume that the interaction potential fundamentally dictates the ranking plot. While this is partly true, only a strictly linear energy distribution yields no peak in the heat capacity. The characteristic S-shaped energy distribution responsible for a peak arises from combinatorics: in most systems, symmetry dictates that very few configurations exhibit extremely favourable or unfavourable energies, while the majority lie in an intermediate favourability range. Indeed, SAMPLE has been

applied to diverse systems with attractive, repulsive, and complex site-specific interaction potentials, and in all cases, S-shaped energy distributions were observed.[16–19]

## S6 EVALUATION OF THERMODYNAMIC PROPERTIES

Determining most observables in the grand canonical picture is relatively straightforward. However, the heat capacity is non-trivial. For the derivation, we start with the expression for the energy. The number of particles  $N$  is a function of the temperature and the chemical potential.

$$E(T, V, N) = E(T, V, N(T, \mu)) \quad (4)$$

Taking the derivative with respect to temperature reveals the term that shall become the heat capacity.

$$\left. \frac{\partial \langle E \rangle}{\partial T} \right|_{V, \mu} = \left. \frac{\partial \langle E \rangle}{\partial T} \right|_{N, V} + \left. \frac{\partial \langle E \rangle}{\partial N} \right|_{T, V} \left. \frac{\partial \langle N \rangle}{\partial T} \right|_{V, \mu} \quad (5)$$

We reorder the equation and get the heat capacity.

$$C_V = \left. \frac{\partial \langle E \rangle}{\partial T} \right|_{N, V} \quad (6)$$

$$= \left. \frac{\partial \langle E \rangle}{\partial T} \right|_{V, \mu} - \left. \frac{\partial \langle E \rangle}{\partial N} \right|_{T, V} \left. \frac{\partial \langle N \rangle}{\partial T} \right|_{V, \mu} \quad (7)$$

In the last expression, not all terms can be calculated directly. However, we can rewrite it into a series of terms that can be calculated.

$$\left. \frac{\partial \langle E \rangle}{\partial \mu} \right|_{T, V} = \left. \frac{\partial \langle E \rangle}{\partial N} \right|_{T, V} \cdot \left. \frac{\partial N}{\partial \mu} \right|_{T, V} \Rightarrow \left. \frac{\partial \langle E \rangle}{\partial N} \right|_{T, V} = \frac{\left. \frac{\partial \langle E \rangle}{\partial \mu} \right|_{T, V}}{\left. \frac{\partial N}{\partial \mu} \right|_{T, V}} \quad (8)$$

$$C_V = \left. \frac{\partial \langle E \rangle}{\partial T} \right|_{V, \mu} - \frac{\left. \frac{\partial \langle E \rangle}{\partial \mu} \right|_{T, V}}{\left. \frac{\partial N}{\partial \mu} \right|_{T, V}} \left. \frac{\partial \langle N \rangle}{\partial T} \right|_{V, \mu} \quad (9)$$

Let us now take a detour and look at the derivatives of the partition function. These will become useful later, as they can be substituted into the various terms in equation 9.

$$Z(\beta, \mu, V) = \sum_{N=0}^{\infty} \sum_i e^{-\beta(E_i^{(N)} - \mu N)} \quad (10)$$

### First derivative

$$\frac{\partial \ln Z}{\partial \beta} = \frac{1}{Z} \frac{\partial Z}{\partial \beta} \quad (11)$$

$$= -\frac{1}{Z} \sum_{N, i} (E_i^{(N)} - \mu N) e^{-\beta(E_i^{(N)} - \mu N)} \quad (12)$$

$$= -\langle E - \mu N \rangle \quad (13)$$

$$= -\langle E \rangle + \mu \langle N \rangle \quad (14)$$

$$\langle E \rangle = \frac{\partial \ln \mathcal{Z}}{\partial \beta} + \mu \langle N \rangle \quad (15)$$

Second derivative

$$\frac{\partial^2 \ln \mathcal{Z}}{\partial \beta^2} = \langle (E - \mu N)^2 \rangle - \langle E - \mu N \rangle^2 = \text{Var}(E - \mu N) \quad (16)$$

Particle number

$$\langle N \rangle = \frac{1}{\beta} \frac{\partial \ln \mathcal{Z}}{\partial \mu} = -\frac{1}{\mathcal{Z}} \sum_{N,i} N e^{-\beta(E_i^{(N)} - \mu N)} \quad (17)$$

To derive the solution, we are taking inspiration from 16:

$$\frac{\partial \langle N \rangle}{\partial \beta} = -(\langle N(E - \mu N) \rangle - \langle N \rangle \langle E - \mu N \rangle) = -\text{Cov}(N, E - \mu N) \quad (18)$$

The same strategy allows us to determine the next derivative:

$$\frac{\partial \langle N \rangle}{\partial \mu} = \beta (\langle N^2 \rangle - \langle N \rangle^2) = \beta \cdot \text{Var}(N) \quad (19)$$

Let us now consider the heat capacity. We start with the first term  $\left. \frac{\partial \langle E \rangle}{\partial T} \right|_{V,\mu}$ :

$$\left. \frac{\partial \langle E \rangle}{\partial T} \right|_{V,\mu} = \frac{\partial \beta}{\partial T} \left. \frac{\partial \langle E \rangle}{\partial \beta} \right|_{V,\mu} = \frac{1}{k_B T^2} \left. \frac{\partial \langle E \rangle}{\partial \beta} \right|_{V,\mu} \quad (20)$$

$$\left. \frac{\partial \langle E \rangle}{\partial \beta} \right|_{V,\mu} = \frac{\partial^2 \ln \mathcal{Z}}{\partial \beta^2} + \cancel{\frac{\partial \mu}{\partial \beta} \langle N \rangle} + \mu \frac{\partial \langle N \rangle}{\partial \beta} \quad (21)$$

We assumed that the chemical potential is not dependent on temperature, so the derivative with respect to  $\beta$  is zero.

$$\left. \frac{\partial \langle E \rangle}{\partial \beta} \right|_{V,\mu} = \text{Var}(E - \mu N) - \text{Cov}(N, E - \mu N) \quad (22)$$

$$\left. \frac{\partial \langle E \rangle}{\partial T} \right|_{V,\mu} = \frac{1}{k_B T^2} \left[ \text{Var}(E - \mu N) - \text{Cov}(N, E - \mu N) \right] \quad (23)$$

Now we look at  $\left. \frac{\partial \langle N \rangle}{\partial T} \right|_{V,\mu}$ :

$$\left. \frac{\partial \langle N \rangle}{\partial T} \right|_{V,\mu} = -\frac{1}{k_B T^2} \cdot \text{Cov}(N, E - \mu N) \quad (24)$$

Next, we look at  $\left. \frac{\partial \langle E \rangle}{\partial \mu} \right|_{T,V}$ :

$$\left. \frac{\partial \langle E \rangle}{\partial \mu} \right|_{T,V} = -\frac{\partial^2 \ln \mathcal{Z}}{\partial \mu \partial \beta} + \langle N \rangle + \mu \frac{\partial \langle N \rangle}{\partial \mu} \quad (25)$$

$$\frac{\partial^2 \ln \mathcal{Z}}{\partial \mu \partial \beta} = \frac{\partial}{\partial \beta} \beta \langle N \rangle = \langle N \rangle + \beta \frac{\partial \langle N \rangle}{\partial \beta} = \langle N \rangle - \beta \cdot \text{Cov}(N, E - \mu N) \quad (26)$$

$$\left. \frac{\partial \langle E \rangle}{\partial \mu} \right|_{T, V} = \beta \cdot \text{Cov}(N, E - \mu N) - \mu \cdot \text{Var}(N) \quad (27)$$

Finally, we can put everything together:

$$C_V = \frac{1}{k_B T^2} \left[ \text{Var}(E - \mu N) - \text{Cov}(N, E - \mu N) \right] \quad (28)$$

$$- \frac{\beta \cdot \text{Cov}(N, E - \mu N) - \mu \beta \cdot \text{Var}(N)}{\beta \cdot \text{Var}(N)} \cdot \frac{1}{k_B T^2} \cdot \text{Cov}(N, E - \mu N) \quad (29)$$

$$C_V = \frac{1}{k_B T^2} \left[ \text{Var}(E - \mu N) - \text{Cov}(N, E - \mu N) - \frac{\text{Cov}(N, E - \mu N)^2 - \mu \cdot \text{Var}(N) \cdot \text{Cov}(N, E - \mu N)}{\text{Var}(N)} \right] \quad (30)$$

$$= \frac{1}{k_B T^2} \left[ \text{Var}(E - \mu N) - \frac{\text{Cov}(N, E - \mu N)^2}{\text{Var}(N)} \right] \quad (31)$$

- 
- [1] J. Moreno and J. M. Soler, Optimal meshes for integrals in real-and reciprocal-space unit cells, *Phys. Rev. B* **45**, 13891 (1992).
- [2] P. Wisesa, K. A. McGill, and T. Mueller, Efficient generation of generalized monkhorst-pack grids through the use of informatics, *Phys. Rev. B* **93**, 155109 (2016).
- [3] B. Saunders, *Predicting the Structure and Stability of Compositionally Diverse Materials*, Phd thesis, University of Warwick (2025).
- [4] T. T. Pham, T. N. Pham, V. Chihaiia, Q. A. Vu, T. T. Trinh, T. T. Pham, L. Van Thang, and D. N. Son, How do the doping concentrations of n and b in graphene modify the water adsorption?, *RSC Adv.* **11**, 19560 (2021).
- [5] S. Bu, N. Yao, M. A. Hunter, D. J. Searles, and Q. Yuan, Design of two-dimensional carbon-nitride structures by tuning the nitrogen concentration, *npj Comput. Mater.* **6**, 128 (2020).
- [6] M. Yang, L. Wang, M. Li, T. Hou, and Y. Li, Structural stability and O2 dissociation on nitrogen-doped graphene with transition metal atoms embedded: A first-principles study, *AIP Adv.* **5**, 067136 (2015).
- [7] I. Choudhuri, N. Patra, A. Mahata, R. Ahuja, and B. Pathak, B-n@graphene: Highly sensitive and selective gas sensor, *J. Phys. Chem. C* **119**, 24827 (2015).
- [8] O. Olaniyan, R. Maphasha, M. Madito, A. Khaleed, E. Igumbor, and N. Manyala, A systematic study of the stability, electronic and optical properties of beryllium and nitrogen co-doped graphene, *Carbon* **129**, 207 (2018).
- [9] S. Kattel, P. Atanassov, and B. Kiefer, Stability, electronic and magnetic properties of in-plane defects in graphene: A first-principles study, *J. Phys. Chem. C* **116**, 8161 (2012).
- [10] N. E. Benti, G. A. Tiruye, and Y. S. Mekonnen, Boron and pyridinic nitrogen-doped graphene as potential catalysts for rechargeable non-aqueous sodium-air batteries, *RSC Adv.* **10**, 21387 (2020).
- [11] E. B. Yutomo, F. A. Noor, and T. Winata, Effect of the number of nitrogen dopants on the electronic and magnetic properties of graphitic and pyridinic N-doped graphene – a density-functional study, *RSC Adv.* **11**, 18371 (2021).
- [12] A. P. Bartók, R. Kondor, and G. Csányi, On representing chemical environments, *Phys. Rev. B: Condens. Matter Mater. Phys.* **87**, 184115 (2013).
- [13] S. De, A. P. Bartók, G. Csányi, and M. Ceriotti, Comparing molecules and solids across structural and alchemical space, *Phys. Chem. Chem. Phys.* **18**, 13754 (2016).
- [14] K. K. Huguenin-Dumittan, P. Loche, N. Haoran, and M. Ceriotti, Physics-inspired equivariant descriptors of nonbonded interactions, *J. Phys. Chem. Lett.* **14**, 9612 (2023).
- [15] F. Nogueira, Bayesian optimization: Open source constrained global optimization tool for python (2014), available at <https://github.com/bayesian-optimization/BayesianOptimization>.
- [16] L. Hörmann, A. Jeindl, A. T. Egger, M. Scherbela, and O. T. Hofmann, Sample: Surface structure search enabled by coarse graining and statistical learning, *Comput. Phys. Commun.* **244**, 143 (2019).
- [17] A. Jeindl, J. Domke, L. Hörmann, F. Sojka, R. Forker, T. Fritz, and O. T. Hofmann, Nonintuitive surface self-assembly of functionalized molecules on ag(111), *ACS Nano* **15**, 6723 (2021).

- [18] M. Scherbela, L. Hörmann, A. Jeindl, V. Obersteiner, and O. T. Hofmann, Charting the energy landscape of metal/organic interfaces via machine learning, *Phys. Rev. Mater.* **2**, 043803 (2018).
- [19] L. Hörmann, A. Jeindl, and O. T. Hofmann, From a bistable adsorbate to a switchable interface: tetrachloropyrazine on pt (111), *Nanoscale* **14**, 5154 (2022).
- [20] J. Lee, W.-C. Tian, W.-L. Wang, and D.-X. Yao, Two-Dimensional Pnictogen Honeycomb Lattice: Structure, On-Site Spin-Orbit Coupling and Spin Polarization, *Sci. Rep.* **5**, 11512 (2015).
